# Supplementary material for: A Coarse-to-Fine Pseudo-Labeling (C2FPL) Framework for Unsupervised Video Anomaly Detection
Source: arXiv:2310.17650 source file (2023-10-26)

## Residual Self-Attention

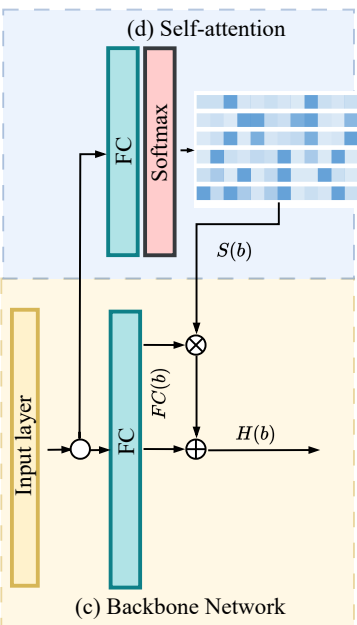

## Multiplicative Self-Attention

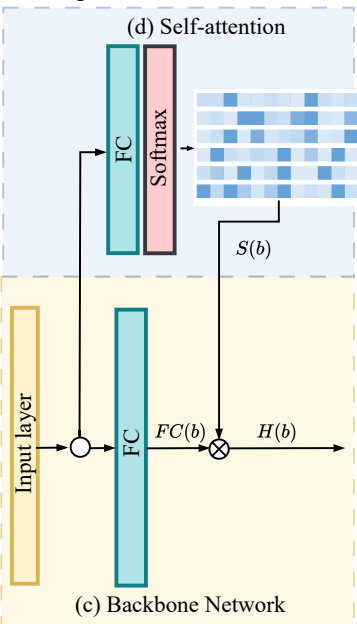

Supplement: Supplementary file 1 [file SA_Final_crop.pdf]
